# Supplementary material for: Path-Based Formulations for the Design of On-demand Multimodal Transit Systems with Adoption Awareness
Source: arXiv:2301.07292 source file (2024-01-31)
Supplement: Supplementary file 12 [file formulation_cpath.tex]

\begin{figure}[!t]
\begin{subequations}
\label{eq_cpath}
\begin{alignat}{1}
\min_{z_{hl}} \quad & \sum_{h,l \in H} \beta_{hl} z_{hl} + \sum_{r \in T_{core}} p^r g^r + \sum_{r \in T_{latent}} \sum_{\pi \in A^r} p^r \lambda^r_\pi (g(\pi)  - \varphi) 
\label{eq_cpath:obj_func} \\
% %%%%%%%%%%%%%%%%%%%%%%%%%%%%%%%%%%%%%%%%%%%%%%%%%%%%%%
% \text{s.t.} \quad & \sum_{l \in H} z_{hl} = \sum_{l \in H} z_{lh} \quad \forall h \in H  
% \label{eq_cpath:bus_flow_balance} \\
% %%%%%%%%%%%%%%%%%%%%%%%%%%%%%%%%%%%%%%%%%%%%%%%%%%%%%%
% & z_{hl} = 1 \quad \forall (h, l) \in Z_{fixed} \label{eq_cpath:fixed_arc} \\
% %%%%%%%%%%%%%%%%%%%%%%%%%%%%%%%%%%%%%%%%%%%%%%%%%%%%%%
% & g^r = \sum_{h,l \in H} \tau_{hl}^r x_{hl}^r + \sum_{i,j \in N} \gamma_{ij}^r y_{ij}^r \quad \forall r \in T_{core} \label{eq_cpath:grDefinition} \\
% %%%%%%%%%%%%%%%%%%%%%%%%%%%%%%%%%%%%%%%%%%%%%%%%%%%%%%
% & \sum_{\substack{h \in H \\ \text{if } i \in H}} (x_{ih}^r - x_{hi}^r) + \sum_{i,j \in N}  (y_{ij}^r - y_{ji}^r) = \begin{cases}
%  1 & \text{if  } i = or^r \\
% -1 & \text{if  } i = de^r \\
% 0 & \text{otherwise}
% \end{cases} \quad \forall i \in N, r \in T_{core} \label{eq_cpath:minFlowConstraint} \\
% %%%%%%%%%%%%%%%%%%%%%%%%%%%%%%%%%%%%%%%%%%%%%%%%%%%%%%
% & x_{hl}^r \leq z_{hl} \quad \forall h,l \in H, r \in T_{core} \label{eq_cpath:openFacilityOnlyAvailable} \\
& \eqref{eq_cpath_hl:bus_flow_balance}-\eqref{eq_cpath_hl:openFacilityOnlyAvailable} \notag \\
%%%%%%%%%%%%%%%%%%%%%%%%%%%%%%%%%%%%%%%%%%%%%%%%%%%%%%
 &   f_\pi^r \leq z_{hl} \quad \forall r \in T_{latent}, \pi \in \Pi^r, (h,l) \in x(\pi) \\
&   \sum\limits_{(h,l) \in x(\pi)} z_{hl} - |x(\pi)| + 1 \leq f^r_{\pi} \quad \forall r \in T_{latent}, \pi \in \Pi^r \\
& f^r_\pi \rightarrow m^r \leq g(\pi) \quad \forall r \in T_{latent}, \pi \in \Pi^r \\
& \lambda_\pi^r \leq f_\pi^r \quad \forall r \in T_{latent}, \pi \in \Pi^r \\
& \lambda^r_\pi \rightarrow m^r \geq g(\pi) \quad \forall r \in T_{latent}, \pi \in \Pi^r \\
%%%%%%%%%%%%%%%%%%%%%%%%%%%%%%%%%%%%%%%%%%%%%%%%%%%%%%
% & \sum\limits_{\pi \in \Pi^r} \lambda_\pi^r = 1 \quad \forall r \in T_{latent} \label{eq_cpath:must_take_1_path} \\
% %%%%%%%%%%%%%%%%%%%%%%%%%%%%%%%%%%%%%%%%%%%%%%%%%%%%%%
% & z_{hl}, x_{hl}^r, y_{ij}^r \in \{0, 1\} \quad \forall h,l \in H, i,j \in N, r \in T_{core} \label{eq_cpath:binaryConstraint_start} \\
% %%%%%%%%%%%%%%%%%%%%%%%%%%%%%%%%%%%%%%%%%%%%%%%%%%%%%%
% &  \lambda_{\pi}^r, f_\pi^r  \in \{0, 1\} \quad  \forall r \in T_{latent}, \pi \in \Pi^r \label{eq_cpath:binaryConstraint_end} 
& \eqref{eq_cpath_hl:must_take_1_path}-\eqref{eq_cpath_hl:binaryConstraint_end} \notag
\end{alignat}
\end{subequations}
\caption{The {\tt C-Path} Formulation.}
\label{fig:c-path}
\end{figure}
